# Supplementary material for: Using machine learning to parameterize moist convection: potential for modeling of climate, climate change and extreme events
Source: arXiv:1806.11037 ancillary file (2018-09-28)
Supplement: Supplementary file 1 [file supporting_information.pdf]

# Supporting Information for "Using machine learning to parameterize moist convection: potential for modeling of climate, climate change and extreme events"

Paul A. O'Gorman[1], John G. Dwyer[1] *

**Contents of this file**

1. Figures S1 to S13

---

Corresponding author: P. A. O'Gorman Department of Earth, Atmospheric and Planetary Sciences, Massachusetts Institute of Technology, Cambridge, Massachusetts 02139, USA. (pog@mit.edu)

[1]Department of Earth, Atmospheric and Planetary Sciences, Massachusetts Institute of Technology, Cambridge, Massachusetts 02139, USA.

*Current address: Dia&Co, New York

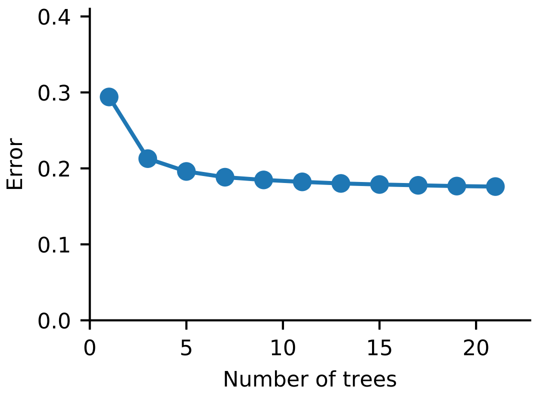


**Figure S1.** Error of the RF trained on the control climate as a function of the number of trees in the ensemble (*n_estimators*). The error is measured by 1-$R^2$, and it is estimated using 10-fold cross-validation on the training dataset. The other hyper-parameters are at their default values of *min_sample_leaf*=10 and *n_train*=$700,000$.

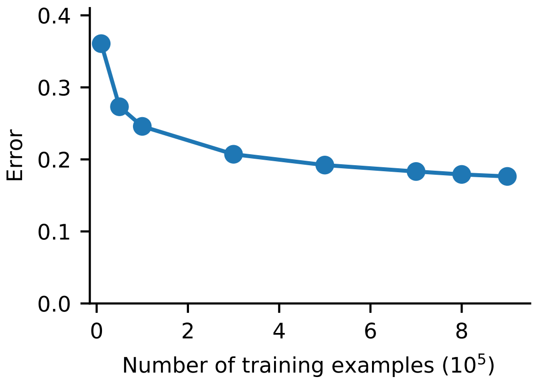


**Figure S2.** As in Fig. S1 but showing the error as a function of the number of training samples used (*n_train*). The minimum value of *n_train* shown is 10,000. The other hyper-parameters are at their default values of *min_sample_leaf*=10 and *n_estimators*=10.

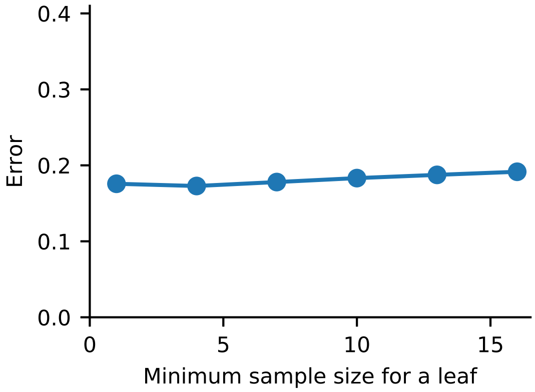


**Figure S3.** As in Fig. S1 but showing the error as a function of the minimum number of training samples required to be at each leaf node (*min_sample_leaf*). The other hyper-parameters are at their default values of *n_esimators*=10 and *n_train*=700,000.

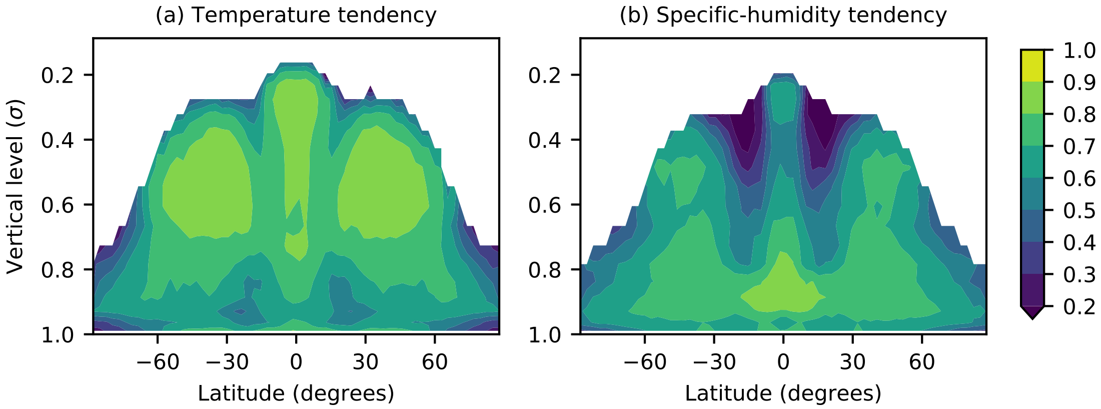


**Figure S4.** As in Fig. 1 but for the $R^2$ of the RF trained on the warm climate applied to the test dataset from the warm climate.

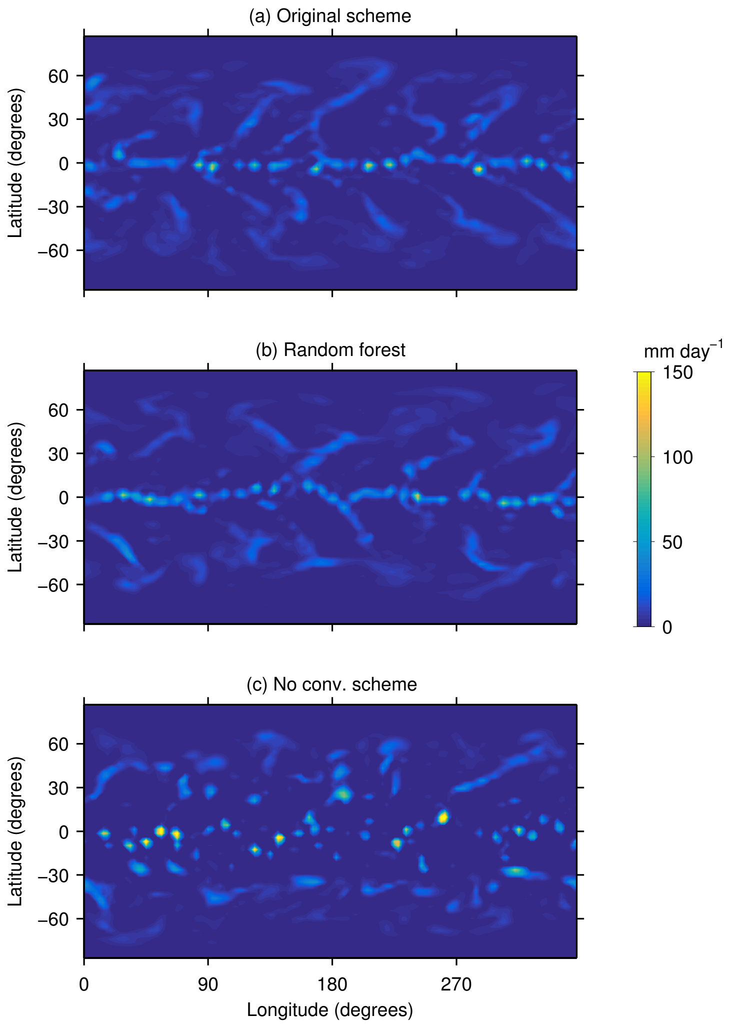


**Figure S5.** Example snapshots of daily precipitation from simulations of the control climate with (a) the RAS convective parameterization, (b) the RF parameterization, and (c) no convection scheme. Total precipitation is shown in each case (including large-scale and convective contributions). The colorbar is saturated at 150 mm day$^{-1}$. Note that these are snapshots from freely running simulations and should not be expected to agree in detail.

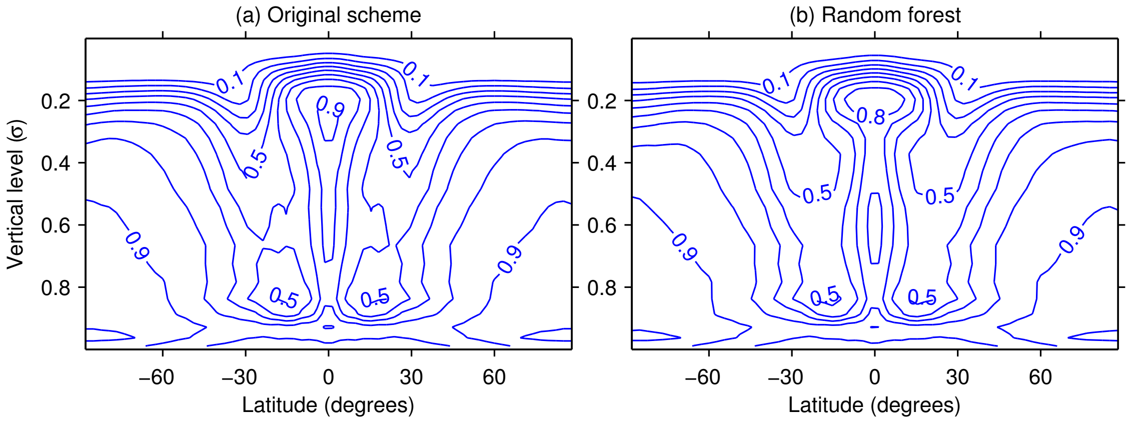


**Figure S6.** Zonal- and time-mean relative humidity versus latitude and vertical level ($\sigma$) in the control climate for simulations with (a) the RAS parameterization and (b) the RF parameterization. The contour interval is 0.1. The difference between results shown in (a) and (b) over all latitudes and levels has a maximum absolute value of 0.18 and a root-mean-square value of 0.04.

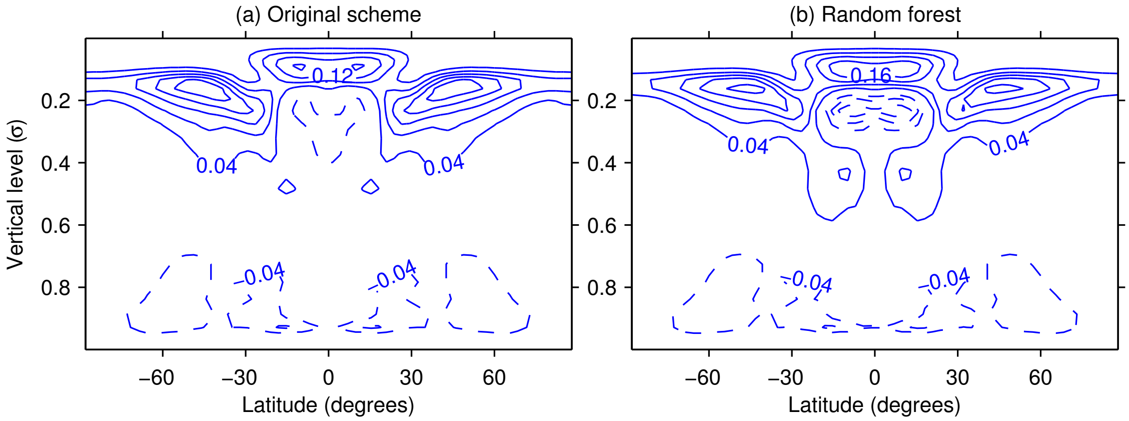


**Figure S7.** As in Fig. 5, but showing the response to climate change of relative humidity. The contour interval is 0.04 and negative contours are dashed. The difference between results shown in (a) and (b) over all latitudes and levels has a maximum absolute value of 0.11 and a root-mean-square value of 0.02.

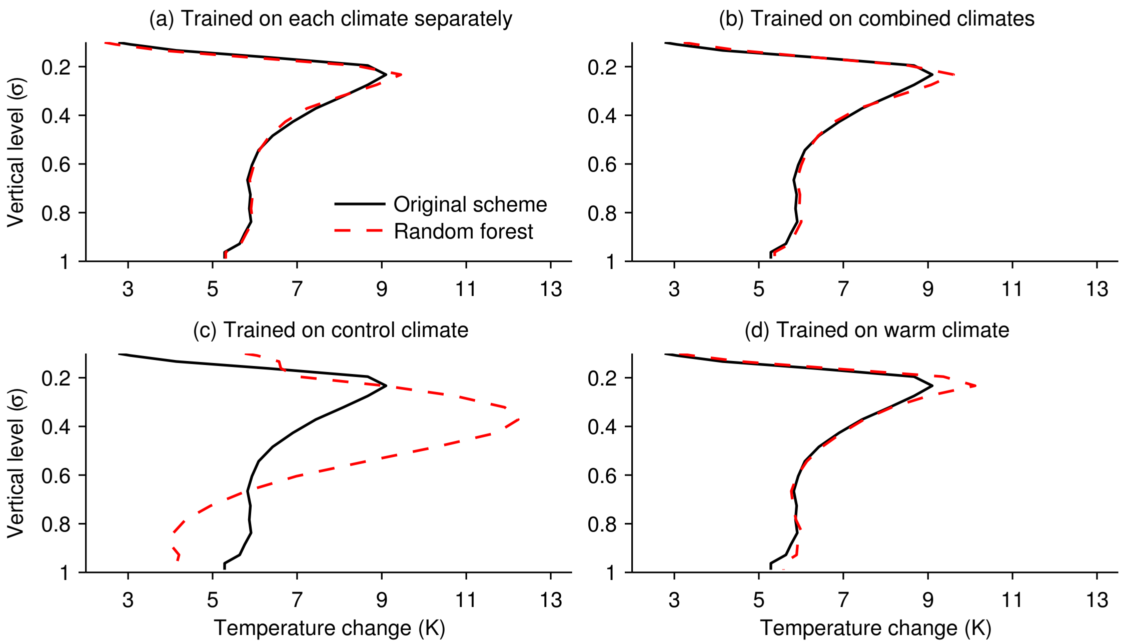


**Figure S8.** The impact of training on different climates on the response to climate change as in Fig. 6, but here showing the mean tropical warming (averaged over 20°S to 20°N) as a function of vertical level $\sigma$.

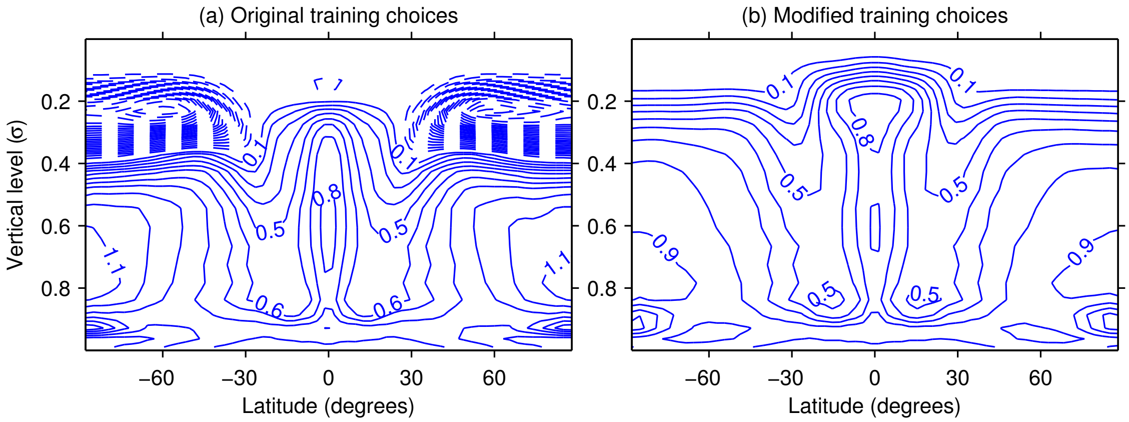


**Figure S9.** Impact of training choices on simulations in which the RF replaces both the moist-convection and large-scale condensation schemes. Shown are the zonal- and time-mean relative humidity in the control climate when: (a) specific humidity is used as the humidity feature, the output scaling for the specific humidity tendency is $L$, and the sampling is weighted by cosine latitude, (b) relative humidity is used as the humidity feature, the output scaling of the specific humidity tendency is $L\sigma^{-3}$, and sampling is not weighted by cosine latitude. The contour interval is 0.1 and negative contours are dashed.

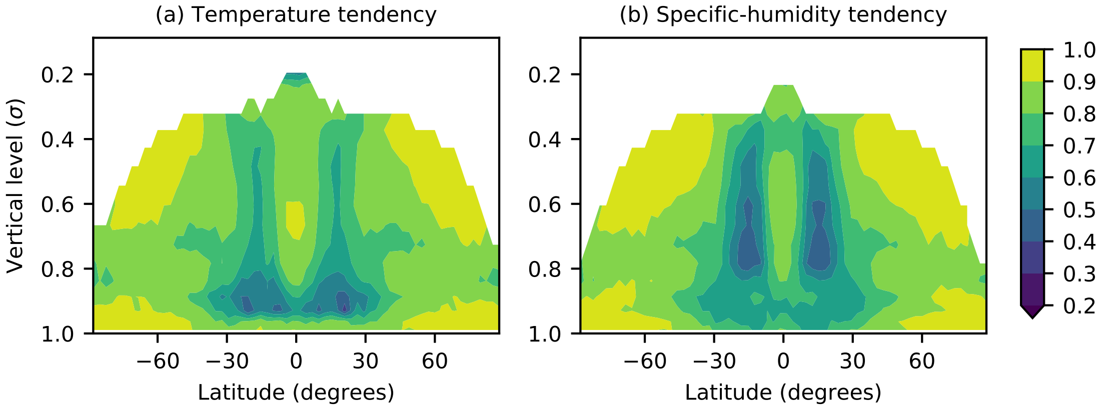


**Figure S10.** As in Fig. 1, but for the RF trained to predict the sum of the tendencies from the moist convection scheme and the large-scale condensation scheme.

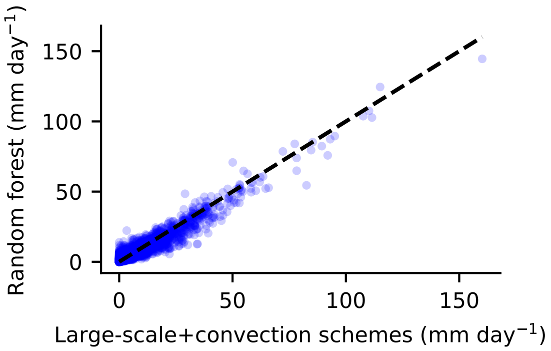


**Figure S11.** As in Fig. 2, but using the RF to predict the sum of the precipitation from the moist convection scheme and the large-scale condensation scheme. $R^2$ is 0.93 and the mean bias is $-3 \times 10^{-2}$ mm day$^{-1}$.

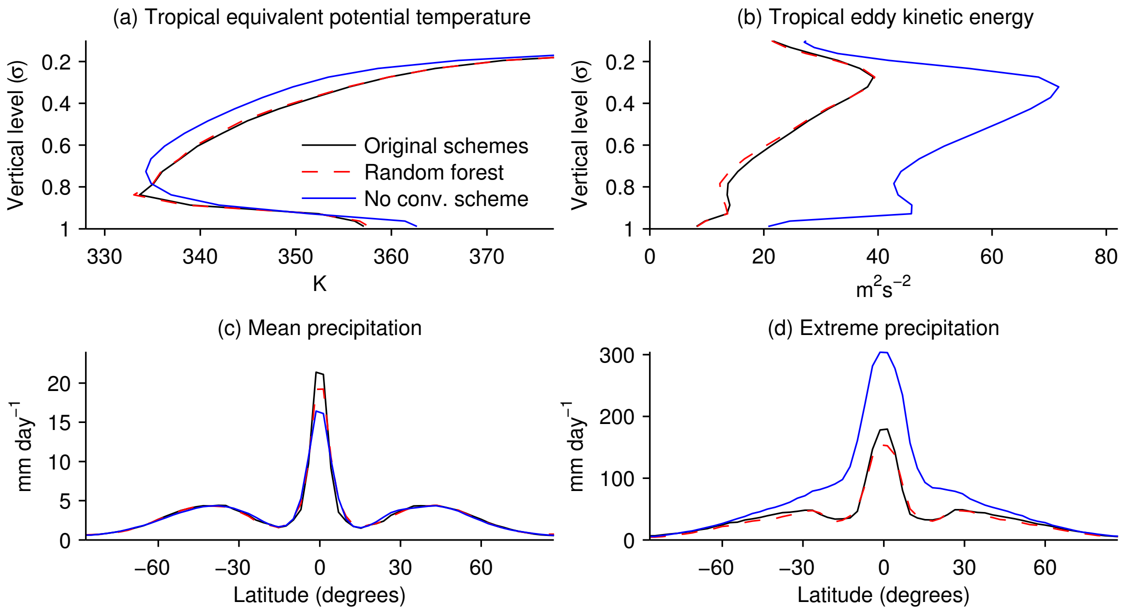


**Figure S12.** As in Fig. 3, but the RF in the GCM replaces both the moist convection scheme and the large-scale condensation scheme.

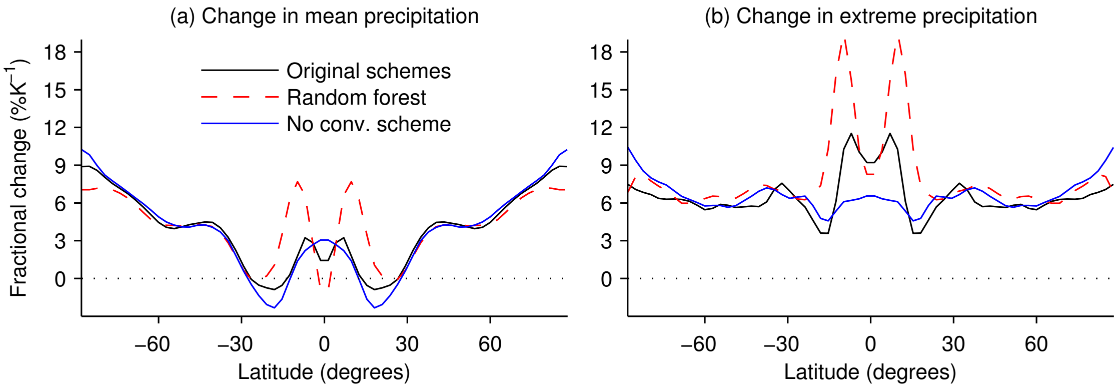


**Figure S13.** As in Fig. 4, but the RF in the GCM replaces both the moist convection scheme and the large-scale condensation scheme.
